# Supplementary material for: Ab Initio Cycloidal and Chiral Magnetoelectric Responses in Cr$_{2}$O$_{3}$
Source: arXiv:1603.00665 source file (2016-09-29)
Supplement: Supplementary file 1 [file si_20160226_NT.pdf]

# Supplementary Material for *Ab Initio* Cycloidal and Chiral Magnetoelectric Responses in $Cr_2O_3$

Natalie Tillack* and Jonathan R. Yates
*Department of Materials, University of Oxford, Oxford, OX1 3PH, United Kingdom*

Paolo G. Radaelli
*Department of Physics, University of Oxford, Oxford, OX1 3PU, United Kingdom*

(Dated: February 26, 2016)

The Supplementary Material consists of two parts: It gives the computational details and illustrates the choice of DFT parameters, as well as a comparison to literature values of magnetoelectric (ME) and ground state properties.

## COMPUTATIONAL DETAILS

We employed the DFT code VASP [1] using projector augmented wave (PAW) potentials [2]. For the Cr atoms, we treated the $3d$ and $4s$ electrons as valence, for O the $2s$ and $2p$ electrons. The plane wave basis set was cut off for energies above 550 eV and a $4\times4\times4$ Monkhorst-Pack grid centred around $\Gamma$ [3] guarantee convergence of the total energy and magnetisation of 0.1 meV and $10^{-5}\,\mu_B$, respectively. We employed the local density approximation (LDA) and the generalised gradient approximation (GGA) with its implementation by Perdew, Burke, and Ernzerhof (PBE) [4]. Blöchl's corrections for the tetrahedron smearing method were employed with a broadening width of 0.05 eV. The structures were relaxed with the conjugated gradient algorithm; a tight convergence criterion of $5\times10^{-6}\,\mathrm{eV\,Å^{-2}}$ had to be chosen to account for the sensitive response of the forces to the magnetic field. No symmetry constraints were used for the calculations.

The BEC were computed using both the $\partial\mathbf{P}/\partial\mathbf{u}$ and the $\partial\mathbf{F}/\partial\boldsymbol{\epsilon}$ implementation to verify the numerical accuracy of the calculations. Both finite differences and density functional perturbation theory were tested and led to similar results when computing the FC matrix. The BEC and the FC matrix were calculated for the $\bar{3}'m'$ ground state treating spins collinearly and as spinors, within the collinear and spinor formalism, leading to identical results to the fourth decimal place. Allowing for noncollinear magnetism in $Cr_2O_3$ did not have a significant influence on the BEC and the FC matrix, which was to be expected, as both couple to the lattice and SOC in $Cr_2O_3$ is small. We thus confirmed that collinear calculations are sufficient for the computation of the FC matrix and the BEC. For the computation of the magnetic charges, spin-orbit coupling (SOC) was included, a Zeeman magnetic field applied according to [5], and the Hellman-Feynman forces on each atom computed. By using the same BEC and FC matrix results for all three magnetic phases, we isolated the influence of the magnetic charges.

## COMPARISON TO LITERATURE

The equilibrium parameters of the $\bar{3}'m'$ phase of $Cr_2O_3$ were calculated for both $xc$ functionals and benchmarked against literature values, table I. The differences are well known in DFT: An over- (under-) binding when using LDA (PBE), the magnetic moment increasing when going from LDA to PBE, and the electronic band gap underestimated by both functionals.

TABLE I. Structural, electronic, and magnetic properties of $Cr_2O_3$ using different $xc$ functionals and benchmarked against literature values.

| Details | $a_{\mathrm{Lat}}$ [Å] | $M_{\mathrm{Cr}}$ [$\mu_B$] | $E_{\mathrm{Gap}}$ [eV] |
|---|---|---|---|
| LDA | 5.26 | 2.2 | 0.8 |
| PBE | 5.42 | 2.7 | 1.7 |
| LDA+U, Ref. [6] | 5.37 | 2.8 | 2.8 |
| LDA, Ref. [7] | 5.32 | 2.0 | 1.3 |
| SQUID, Ref. [8] | 5.36 | 2.65 / 2.31 | |

For simplicity, because it provides a more stable implementation with noncollinear magnetism than the GGA functionals, and because it leads to a reasonably good description of the ground state, the results given in the main text are based on our LDA calculations.

We did however repeat the calculations for the ME coupling tensor of the LF $\bar{3}'m'$ phase using PBE and compared to the results in Ref. [9] leading to almost identical results, table II. The results are given in the basis of the IR active phonon modes, which for $Cr_2O_3$ are the four doubly degenerate transverse $E_u$ and two singly degenerate longitudinal $A_{2u}$ modes. We noticed that the differences between GGA and LDA functionals in the strength of the ME coupling are mainly attributed to the different lattice constant that both functionals predict.

From the mode decomposition of the BEC and the magnetic charges in the two SF phases, we observe changes in the magneto-active response due to $x$ and $y$ no longer being equivalent. The degeneracy of the IR

TABLE II. Comparison of the mode decomposed Born effective charges (in $e$), magnetic charges (in $10^{-2}\,\mu_B/\text{Å}$), the overall ME coupling tensor (in $\text{ps}\,\text{m}^{-1}$), and the respective eigenvalues of the FC matrix $C_n$ (in $\text{eV}/\text{Å}^2$) for the $\bar{3}'m'$ phase of $Cr_2O_3$ compared to Ref. [9]. The PBE functional was used in both cases.

| Mode | PBE | | | | PBE, Ref. [9] | | | |
|---|---|---|---|---|---|---|---|---|
| | $Z^e$ | $Z^m$ | $C$ | $\alpha$ | $Z^e$ | $Z^m$ | $C$ | $\alpha$ |
| ${E_u}^1$ | 6.8 | 9.5 | 29 | 0.263 | 7.1 | 10.6 | 31 | 0.290 |
| ${E_u}^2$ | 3.8 | 14.9 | 19 | 0.361 | 3.7 | 16.1 | 20 | 0.356 |
| ${E_u}^3$ | 0.2 | -3.7 | 15 | -0.005 | 0.4 | -4.0 | 16 | -0.012 |
| ${E_u}^4$ | 0.8 | -0.0 | 10 | 0.000 | 0.6 | -0.8 | 10 | -0.005 |
| All $\perp$ | | | | 0.618 | | | | 0.629 |
| ${A_{2u}}^1$ | 8.6 | 0.1 | 21 | 0.003 | 8.5 | 0.1 | 23 | 0.002 |
| ${A_{2u}}^2$ | 1.0 | 0.0 | 10 | 0.001 | 1.2 | 0.0 | 11 | 0.000 |
| All $\parallel$ | | | | 0.004 | | | | 0.003 |

active $E_u$ modes is removed, and other modes become magneto-active in $x$, $y$, or $z$. We also find that the exceptionally large component in the $Z^m$(Cr) (the 32 and 31 component in the $2'/m$ and $2/m'$ phase, respectively; results given in the main text) maps onto magneto-active modes that are mutually exclusive to the IR active ones. That value has therefore no effect on the coupling tensor, explaining why – despite the magnetic charge tensors being quite different in the LF and SF cases – in all three coupling tensors related elements have similar numerical values.

* natalie.tillack@materials.ox.ac.uk

[1] G. Kresse and J. Furthmüller, Physical Review B - Condensed Matter and Materials Physics B, Condensed matter **54**, 11169 (1996).
[2] P. E. Blöchl, Physical Review B **50**, 17953 (1994).
[3] H. J. Monkhorst and J. D. Pack, Physical Review B **13**, 5188 (1976).
[4] J. Perdew, K. Burke, and M. Ernzerhof, Physical review letters **77**, 3865 (1996).
[5] E. Bousquet and N. A. Spaldin, Physical Review Letters **107**, 1 (2011).
[6] N. J. Mosey, P. Liao, and E. A. Carter, The Journal of chemical physics **129**, 014103 (2008).
[7] S. Coh, D. Vanderbilt, A. Malashevich, and I. Souza, Physical Review B **83**, 85108 (2011).
[8] A. H. Hill, A. Harrison, C. Dickinson, W. Zhou, and W. Kockelmann, Microporous and Mesoporous Materials **130**, 280 (2010).
[9] M. Ye and D. Vanderbilt, Physical Review B **89**, 064301 (2014).
